# Supplementary material for: Stochastic Reweighted Gradient Descent
Source: arXiv:2103.12293 source file (2021-03-23)
Supplement: Supplementary file 1 [file review_sgd.tex]

Before we give the proofs of the main results
that study the convergence of SRG, we review here
the standard analysis of SGD. This will allow
us to compare the performance of SGD and SRG.
Recall that SGD uses the following recurrence relation:
\begin{equation}
    x_{k+1} = x_k - \alpha_k \nabla f_{i_k}(x_k)
    \label{SGD}
\end{equation}
where $i_k$ is uniformly distributed on $[n]$.

The main result of the analysis of SGD is the following
Theorem:
\begin{theorem}
    Suppose that Assumptions \ref{strongly-convex},
    \ref{convex}, and \ref{smooth} hold,
    and that $x_k$ evolves according to (\ref{SGD})
    with $\alpha_k \leq 1/2L$.
    Then:
    \begin{equation*}
        \E{\sqnorm{x_{k+1} - \xstar}} \leq 
        (1-\alpha_k\mu) \E{\sqnorm{x_k - \xstar}} + 2 \alpha_k^2 \sigma^2
    \end{equation*}
    \label{sgd_one_step}
\end{theorem}
\begin{proof}
    Taking expectation with respect to $i_k$ conditional on $(i_t)_{t=1}^{k-1}$
    we have:
    \begin{align*}
        &\E{\sqnorm{x_{k+1} - \xstar}} \\
        &= \E{\sqnorm{x_{k} - \alpha_k \nabla f_{i_k}(x_k) - \xstar}} \\
        &= \sqnorm{x_k - \xstar} - 
        2 \alpha_k \inp{\E{\nabla f_{i_k}(x_k)}}{x_k - \xstar} +
        \alpha_k^2 \E{\sqnorm{\nabla f_{i_k}(x_k)}} \\
        &\leq \sqnorm{x_k - \xstar} -
        2 \alpha_k \inp{\nabla F(x_k)}{x_k - \xstar} +
        2 \alpha_k^2 \E{\sqnorm{\nabla f_{i_k}(x_k) - \nabla f_{i_k}(\xstar)}} +
        2 \alpha_k^2 \E{\sqnorm{\nabla f_{i_k}(\xstar)}} \\
        &\leq (1 - \alpha_k\mu) \sqnorm{x_k - \xstar} +
        2 \alpha_k^2 \sigma^2 +
        2 \alpha_k \left(2L\alpha_k - 1\right) \left[F(x_k) - F(\xstar)\right]
    \end{align*}
    where the fourth line follows from Proposition \ref{youngs_inequality},
    and the fifth line from the definition of $\sigma^2$ in
    section \ref{convergence}, Assumption \ref{strongly-convex}
    (strong-convexity of F) applied to the inner product term,
    and Lemma \ref{grad_norm_bound} applied to the remaining term.
    For $\alpha_k \leq 1/2L$ the third term is negative, so
    that taking total expectation on both sides yields the result.
\end{proof}

The above Theorem leads to the following convergence
rate for SGD with a constant step size.
\begin{corollary}
    Under the assumptions of Theorem \ref{sgd_one_step},
    and using a constant step size $\alpha \leq 1/2L$,
    we have for any $k \in \mathbb{N}$:
    \begin{equation*}
        \E{\sqnorm{x_k - \xstar}} \leq 
        (1 - \alpha \mu)^k \sqnorm{x_0 - \xstar}
        +
        \frac{2\alpha \sigma^2}{\mu}
    \end{equation*}
\end{corollary}
\begin{proof}
    Starting from $\sqnorm{x_k - \xstar}$ and alternating
    taking expectation and applying Theorem \ref{sgd_one_step}
    we get:
    \begin{align*}
        \E{\sqnorm{x_k - \xstar}} 
        &\leq
        (1-\alpha \mu)^k \sqnorm{x_0 - \xstar}
        + 2\alpha^2 \sigma^2 \sum_{t=0}^{k-1} (1-\alpha\mu)^t \\
        &\leq
        (1 - \alpha\mu)^k \sqnorm{x_0 - \xstar}
        + 2\alpha^2 \sigma^2 \sum_{t=0}^{\infty} (1-\alpha\mu)^t \\
        &= (1 - \alpha\mu)^k \sqnorm{x_0 - \xstar}
        + \frac{2\alpha\sigma^2}{\mu}
    \end{align*}
\end{proof}

For decreasing step sizes, we have the following result:
\begin{corollary}
    Under the assumptions of Theorem \ref{sgd_one_step},
    and using the step sizes:
    \begin{equation*}
        \alpha_k = \frac{2(k + k_0) + 1}
        {\left[c + (k+k_0)(k+k_0+2)\right]\mu}
    \end{equation*}
    where:
    \begin{align*}
        k_0 &= \frac{4L}{\mu} - 2 \\
        c &= \frac{2L}{\mu}
    \end{align*}
    Then:
    \begin{equation*}
        \E{\sqnorm{x_k - \xstar}}
        \leq O\left(\frac{\sqnorm{x_0 - \xstar}}{k^2}\right) +
        O\left(\frac{\sigma^2}{k}\right)
    \end{equation*}
\end{corollary}
\begin{proof}
    It is easy to check that $\alpha_0 = 1/2L$,
    and that the sequence $(\alpha_k)_{k=1}^{\infty}$
    is decreasing, so that the step size condition
    of Theorem \ref{sgd_one_step} holds for
    all $k \in \mathbb{N}$. Fix $k \in \mathbb{N}$.
    We have by Theorem \ref{sgd_one_step} for any
    $t \in [k-1]\cup \{0\}$:
    \begin{align*}
        \E{\sqnorm{x_{t+1} - \xstar}} &\leq 
        (1-\alpha_t\mu) \E{\sqnorm{x_{t} - \xstar}} + 
        2\alpha_t^2 \sigma^2 \\[1em]
        &= \frac{c + (t+k_0-1)(t+k_0+1)}{c + (t+k_0)(t+k_0+2)} 
        \E{\sqnorm{x_t - \xstar}}
        + 2\alpha_t^2 \sigma^2
    \end{align*}
    multiplying both sides by \(\left[c + (t+k_0)(t+k_0+2)\right]\) and
    noticing that:
    \begin{equation*}
        \left[c + (t+k_0)(t+k_0+2)\right]\alpha_t^2 = 
        \frac{\left[2 (t + k_0) + 1\right]^2}
        {\left[c + (t+k_0)(t+k_0+2)\right]} \leq 4
    \end{equation*}
    we get:
    \begin{align*}
        \left[c + (t+k_0)(t+k_0+2)\right]\E{\sqnorm{x_{t+1} - \xstar}} - 
        \left[c + (t+k_0-1)(t+k_0+1)\right]\E{\sqnorm{x_{t} - \xstar}}
        \leq 8\sigma_*^2
    \end{align*}
    summing the \(k\) inequalities for \(t \in [k-1] \cup \{0\}\) and noticing
    that the left side is a telescoping sum we obtain:
    \begin{align*}
        \left[c + (k+k_0)(k+k_0+2)\right]\E{\sqnorm{x_k - \xstar}}
        -
        \left[c + (k_0 - 1)(k_0 + 1)\right] \sqnorm{x_0 - \xstar}
        \leq 
        8k\sigma^2
    \end{align*}
    rearranging yields:
    \begin{align*}
        \E{\sqnorm{x_k - \xstar}} \leq 
        \frac{c + (k_0 - 1)(k_0 + 1)}{c + (k+k_0)(k+k_0+2)}
        \sqnorm{x_0 - \xstar} +
        \frac{8k\sigma^2}{c + (k+k_0)(k+k_0+2)}
    \end{align*}
\end{proof}
